# Supplementary material for: Turbulence in the two-dimensional Fourier-truncated Gross-Pitaevskii equation
Source: arXiv:1301.3383 source file (2013-01-15)
Supplement: Supplementary file 1 [file supplementary.pdf]

# Supplementary Material: Turbulence in the Two-dimensional Fourier-truncated Gross-Pitaevskii Equation

Vishwanath Shukla<sup>1</sup>, Marc Brachet<sup>2</sup> and Rahul Pandit<sup>1</sup> ‡

<sup>1</sup> Centre for Condensed Matter Theory, Department of Physics, Indian Institute of Science, Bangalore 560012, India

<sup>2</sup> Laboratoire de Physique Statistique de l'Ecole Normale Supérieure, associé au CNRS et aux Universités Paris VI et VII, 24 Rue Lhomond, 75231 Paris, France

E-mail: vishwanath@physics.iisc.ernet.in, brachet@physique.ens.fr, rahul@physics.iisc.ernet.in

## 1. Video S1

<http://www.physics.iisc.ernet.in/~rahul/movies/ft2dgp-movies/video-S1.mpg>

This video illustrates the time evolutions, from our DNS run A1, of the following: [top left panel] semilog (base 10) plots of the PDFs of the  $x$  (red circles) and  $y$  (green squares) components of the velocity (cf. figure 2 (a)-(c)); [top right panel] pseudocolor plots of the vorticity  $\omega = \nabla \times \mathbf{v}$  (with high- $k$  modes filtered out); [bottom left panel] log-log (base 10) plots of the spectra  $E_{kin}^i(k)$ ,  $E_{kin}^c(k)$ , and  $E_q(k) + E_{int}(k)$  (cf. figures 4 (a), 5 (a)-(c), and 7 (a)-(c); the orange-dashed line shows a  $k$  power-law behaviour); [bottom right panel] log-log (base 10) plots of the spectra  $n(k)$  (cf. figures 8 (a)-(c); a  $k^{-1}$  power law is shown by the orange-dashed line).

## 2. Video S2

<http://www.physics.iisc.ernet.in/~rahul/movies/ft2dgp-movies/video-S2.mpg>

This video illustrates the time evolution of log-log (base 10) plots of the compensated, incompressible kinetic energy spectra  $k^{5/3}E_{kin}^i(k)$  from our DNS runs A1 (purple curve), A2 (green curve), A3 (sky-blue curve), and A4 (brown curve); a  $k^{-5/3}$  power law in  $E_{kin}^i(k)$  is shown by the orange-dashed line to guide the eye (for uncompensated versions of these spectra see figures 4 (a)-(d)).

## 3. Video S3

<http://www.physics.iisc.ernet.in/~rahul/movies/ft2dgp-movies/video-S3.mpg>

‡ Also at Jawaharlal Nehru Centre For Advanced Scientific Research, Jakkur, Bangalore, India

This video illustrates the time evolution of log-log (base 10) plots of the spectrum  $E_{kin}(k)$  from the following DNS runs: [panel V1] - A1 (purple curve), A2 (green curve), and A3 (sky-blue curve); [panel V2] A6 (purple curve), A9 (green curve), and A10 (sky-blue curve); [panel V3] A11 (purple curve), A12 (green curve), and A13 (sky-blue curve); [panel V4] A1 and A5-A8 (with  $N_c^2 = 1024^2, 512^2, 256^2, 128^2$ , and  $64^2$ ).
